# Supplementary material for: High Frequency Nonlinear Response of Superconducting Cavity-Grade Nb surfaces
Source: arXiv:1904.07432 ancillary file (2019-06-13)
Supplement: Supplementary file 1 [file Supp.pdf]

## Supplementary Information

Bakhrom Oripov,<sup>1,\*</sup> Thomas Bieler,<sup>2</sup> Gianluigi Ciovati,<sup>3</sup> Sergio Calatroni,<sup>4</sup> Pashupati Dhakal,<sup>3</sup> Tobias Junginger,<sup>5</sup> Oleg B. Malyshev,<sup>6</sup> Giovanni Terenziani,<sup>4</sup> Anne-Marie Valente-Feliciano,<sup>3</sup> Reza Valizadeh,<sup>6</sup> Stuart Wilde,<sup>6</sup> and Steven M. Anlage<sup>1</sup>

<sup>1</sup>*Center for Nanophysics and Advanced Materials, Department of Physics,  
University of Maryland, College Park, MD 20742, USA*

<sup>2</sup>*Chemical Engineering and Materials Science, Michigan State University, East Lansing, Michigan 48824, USA*

<sup>3</sup>*Thomas Jefferson National Accelerator Facility, Newport News, Virginia 23606, USA*

<sup>4</sup>*European Organization for Nuclear Research (CERN), 1211 Geneva 23, Switzerland*

<sup>5</sup>*Engineering Department, Lancaster University, Lancaster LA1 4YW, United Kingdom*

<sup>6</sup>*ASTeC, STFC Daresbury Laboratory, Warrington WA4 4AD, United Kingdom*

(Dated: April 15, 2019)

This is the supplementary information for the "High Frequency Nonlinear Response of Superconducting Cavity grade Nb surfaces" article. The document contains three sections:

(A) Experimental Procedure and Data Analysis

In this section, the experimental setup and data acquisition procedure are described in detail.

(B) Resistively Shunted Junction (RSJ) Model and Scale Factors

In this section, the RF current-biased RSJ model, numerical calculation strategy and the fitting procedure are described in detail.

(C) Time-Dependent Ginzburg-Landau (TDGL) Model

In this section, the TDGL model, vortex semi-loops and harmonic response generated by this process are briefly described.

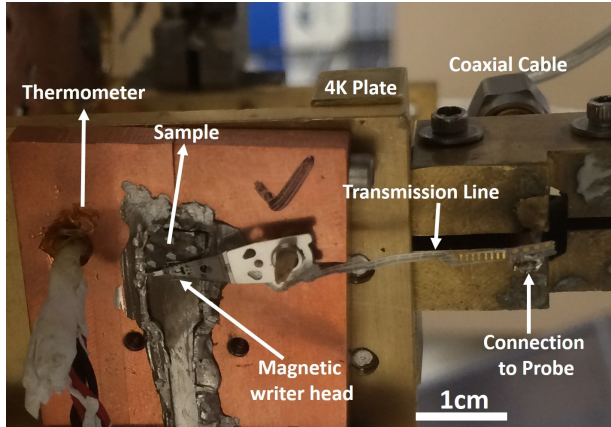

FIG. S1. Photograph of the Experimental setup. The magnetic writer head is connected to an SMA coaxial connector by directly soldering it to the pads on the end of writer probe's transmission line. The Nb sample is attached to the cold plate of an Entropy 4K L-series cryostat. The probe is in direct contact with the sample in this case.

### A. EXPERIMENTAL PROCEDURE AND DATA ANALYSIS

Fig.S1 shows a photograph of the experimental setup. A large grain bulk Nb sample provided by the Bieler group (MSU) is attached to the cold plate of the cryostat. A custom made copper holder is used to firmly hold the sample, and the gap between the sample and the cop-

per holder is filled with indium foil. The data from this measurement is shown in Figs. 2 and 3 in the main text.

Another set of bulk Nb samples were provided by the Ciovati group at Jefferson Lab. A high purity fine-grain niobium sheet was cut into small samples by wire electrodischarge machining. Later these samples were etched using buffered chemical polishing, heat treated at 600°C and etched again. Afterwards, the samples were nanopolished to obtain a surface with mirror quality smoothness. Further details of sample preparation and characterization are available in ref. [1]. The data from this sample is very similar to data obtained from large grain bulk Nb sample. Fig.S2 shows representative nonlinear response data from sample "F9" mentioned in [1].

A set of Nb on copper thin-film samples were provided by the Malyshev group at Accelerator Science and Technology Centre (ASTeC). Four samples were deposited by high-power impulse magnetron sputtering (HIPIMS) at 700°C and various bias voltages on the Cu substrate [2]. All Nb films have a thickness of 1.3 $\mu$ m. A very similar periodic response of  $V_{3f}$  vs  $H_{rf}$  is observed. Fig.S3 shows representative nonlinear response data from one of those samples.

A set of Nb thin films were provided by the Valente-Feliciano group at Jefferson Lab. The sample was coated with continuous ion energy of 184 eV and has a thickness of 570 nm [3]. Fig. S4 shows representative nonlinear response data from this sample. In this case, fifth harmonic response  $V_{5f}$  was measured, and a very similar periodic response of  $V_{5f}$  vs  $H_{rf}$  is observed. A similar behaviour of  $V_{5f}$  was observed in the CERN film. We have found

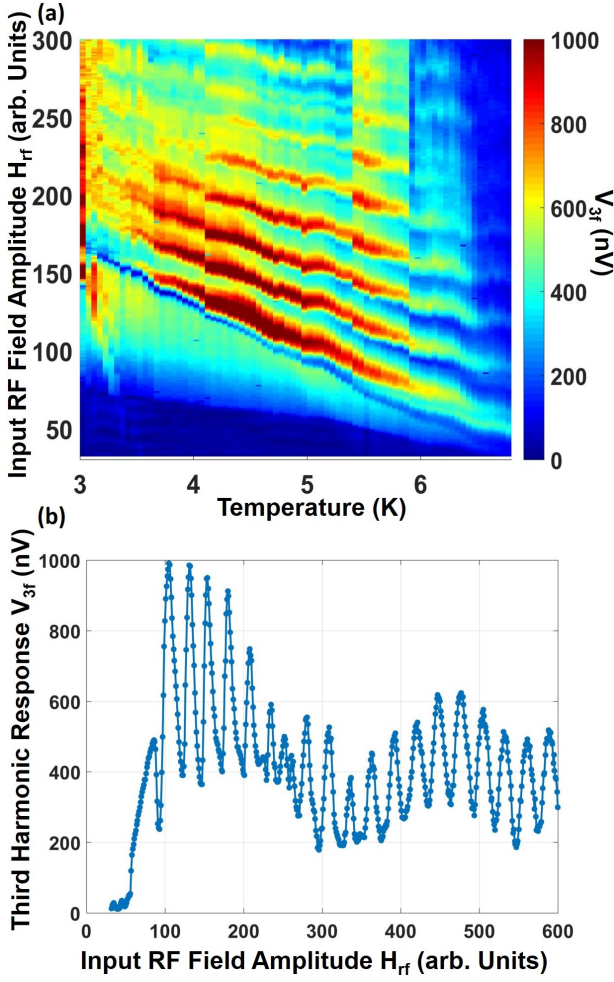

FIG. S2. (a) Small grain bulk Nb third harmonic data vs temperature and applied RF field amplitude measured at 5.07 GHz RF input frequency. The sample was provided by G. Ciovati at Jefferson Lab. (b) vertical line cut through this image ( $V_{3f}$  vs  $H_{rf}$ ) at a constant temperature of  $T=5.0$  K.

that the driven RSJ model shows dips in  $V_{5f}$  at the same  $H_{rf}$  as  $V_{3f}$ .

The data from all these samples is very similar to those in Figs. 2,3 and 4 in the main text. The fact that such a wide variety of Nb samples produce similar response indicates that this is a generic response of air-exposed Nb surfaces.

Concerning Fig.2 of the main text, to analyze the temperature dependence of the periodic response, the RF field amplitudes corresponding to the dips in  $V_{3f}(H_{rf})$  were identified and defined as  $H_{pn}(T)$  where  $n$  stands for  $n$ 'th dip and  $T$  is the temperature of the measurement (Fig.S5). We find that  $H_{pn}$  decreases linearly with increasing temperature and reaches a finite saturation value at  $T_c$ . Furthermore, to link the experimental data with the outcome of the current-biased RSJ model, all

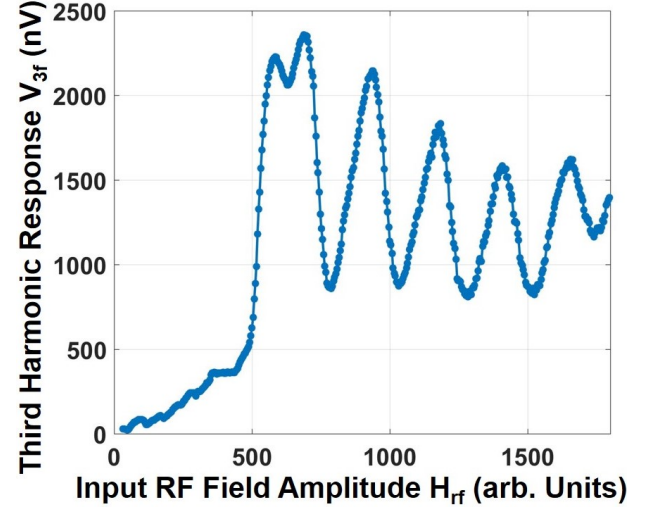

FIG. S3. Third harmonic response  $V_{3f}$  vs input RF field amplitude  $H_{rf}$  data at 7.5K and 4.855 GHz RF input frequency on Nb on Cu. The sample was provided by Oleg Malyshev's group in ASTeC.

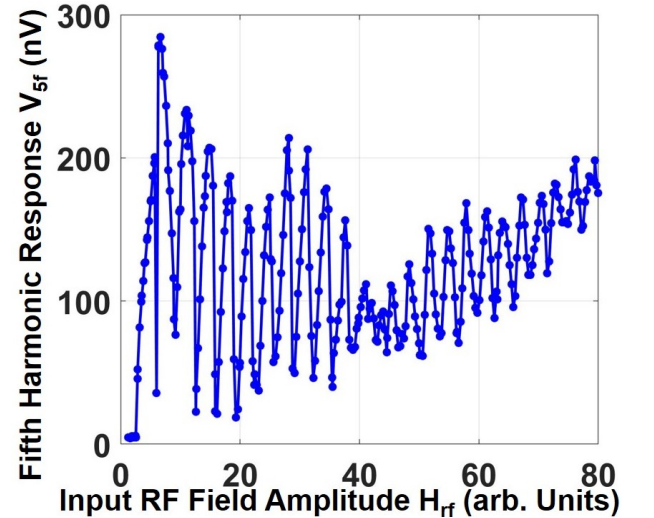

FIG. S4. Fifth harmonic response  $V_{5f}$  vs input RF field amplitude  $H_{rf}$  data at 4.2K and 1.361 GHz RF input frequency on Nb thin film. The sample was provided by A. Valente-Feliciano's group in Jefferson Lab.

dips  $H_{pn}(T)$  are fitted to a straight line, then the slope of the line is defined as "period" and the y-intercept is defined as onset of periodicity  $H_{p0}(T)$  (Fig.S6).

Also we can see 3 separate families of dips which can be attributed to 3 separate weak-links (Fig.S5 and Fig.2 in the main text). Table S.I summarizes the fit parameters for these 3 weak-link families. The fit procedure and parameters are presented in part B. Higher scaling factor

$X_{scale} = \frac{I_\omega R}{H_{rf}}$  values presumably correspond to a weak-link being closer to the magnetic writer probe location.

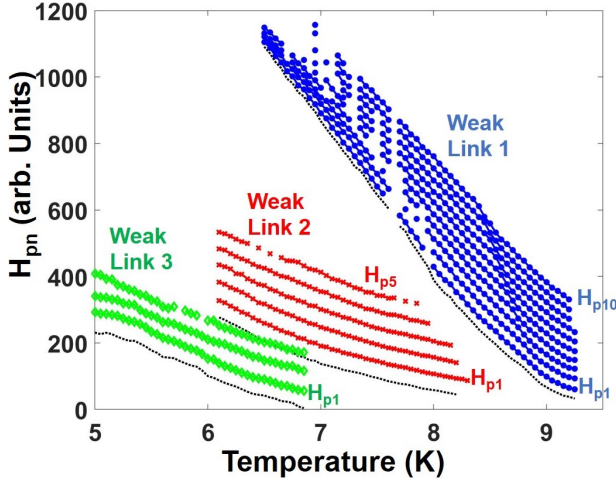

FIG. S5. First few  $H_{pn}$  and the onset of periodicity  $H_{p0}$  (black dashed line) vs temperature for the large grain bulk Nb sample. Three separate families of dips (blue, red, green) can be attributed to 3 separate weak-links. Data from this sample is shown in Figs. 2,3 of the main text.

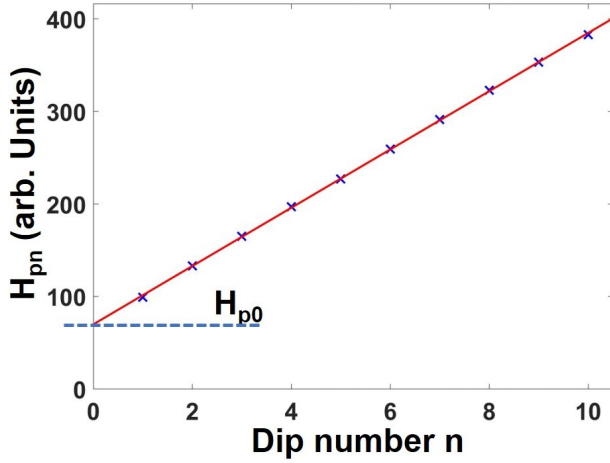

FIG. S6.  $H_{pn}$  vs  $n$  for large grain bulk Nb sample at 9.0K. The solid line is a linear fit to the data.  $H_{p0}$  is defined as the y-intercept of this fit. Period is defined as the slope of the fitted line. In this particular example,  $H_{p0} = 70.1 \text{ arb.units}$  and the period is  $31.54 \text{ arb.units}$ .

## B. RESISTIVELY SHUNTED JUNCTION (RSJ) MODEL and SCALE FACTORS

The response of a small single junction to RF stimulus can be accurately modeled with the RCSJ model [4]. In this model the Josephson junction is modeled as an ideal Josephson junction shunted by a resistance (R) and a capacitance (C) to form a parallel circuit. For very small driving frequency  $2\pi f \ll \omega_p$  compared to plasma frequency of the junction, the model can be simplified

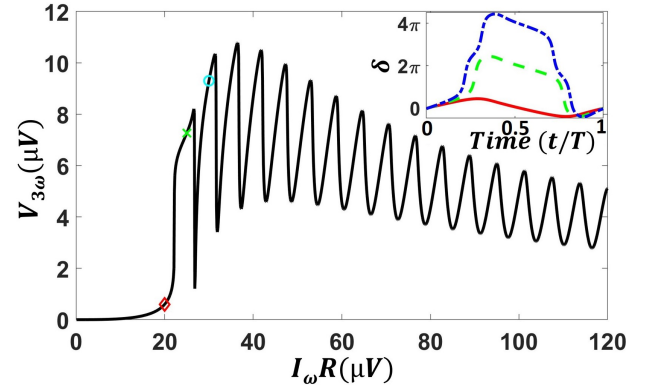

FIG. S7. Calculated third harmonic voltage across an RSJ junction vs  $I_\omega R$  for  $I_c R = 20 \mu V$ . Inset:  $\delta(t)$  across the junction for one RF period in steady state for  $I_\omega R = 20 \mu V$  (red  $\diamond$  - solid line),  $I_\omega R = 25 \mu V$  (green  $\times$  - dashed line) and  $I_\omega R = 30 \mu V$  (blue  $\bullet$  - dot dashed line).

and the capacitive branch can be ignored:

$$I_c \sin \delta + \frac{\Phi_0}{2\pi R} \frac{\partial \delta}{\partial t} + \frac{\Phi_0 C}{2\pi} \frac{\partial^2 \delta}{\partial t^2} = I_\omega \sin(\omega t) \quad (S1)$$

$$V = \frac{\Phi_0}{2\pi} \frac{\partial \delta}{\partial t} \quad (S2)$$

Here  $\delta$  is the gauge-invariant phase difference across the junction and  $V$  is the potential difference across the junction. Eq. S1 can be normalized and rearranged:

$$I_c R \sin \delta + \frac{\Phi_0}{2\pi} \frac{\partial \delta}{\partial t} = I_\omega R \sin(\omega t) \quad (S3)$$

Eq. S3 can be solved for a known  $\omega$ ,  $I_c R$  and  $I_\omega R$  to obtain  $\delta(t)$  and  $V(t)$ . After the solution for  $\delta(t)$  comes to steady state one can take the Fourier transform of  $V(t)$  to calculate the  $3^{rd}$ -harmonic voltage- $V_{3\omega}$  across the junction (Fig. S7).

The harmonic response predicted by the RSJ model, as shown in Fig. S7, is very similar to the data shown in Fig. 3 of the main text. Each peak in  $V_{3\omega}$  vs  $I_\omega R$  corresponds to adding a  $2\pi$  phase-slip across the junction in the driving RF cycle. Note that the separation between the dips as a function of  $I_\omega R$  is constant. This calculation was repeated for all possible values of  $I_c R$ . The challenging part of this model is to relate simulation results to experimental data. From measurements we have  $H_{rf}$  in arbitrary units, while in the RSJ calculation we have the biasing current  $I_\omega R$  in  $\mu V$ . A scaling factor  $X_{scale} = \frac{I_\omega R}{H_{rf}}$  has to be found. Also,  $V_{3\omega}$  is calculated across the junction, while the third harmonic response

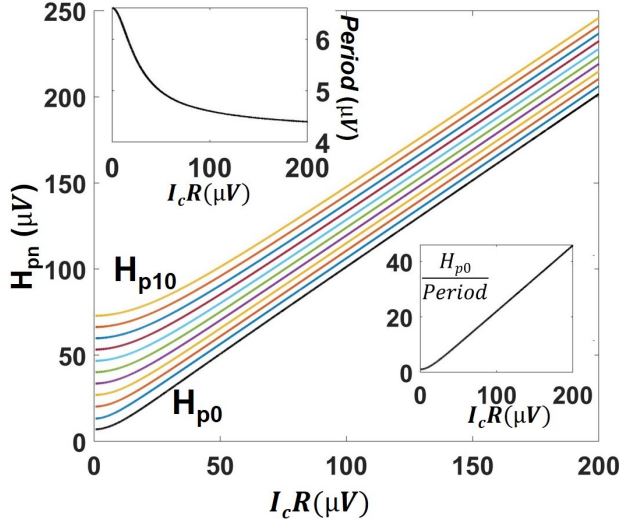

FIG. S8.  $H_{p0}$  to  $H_{p10}$  vs  $I_c R$  calculated from the RSJ model. Top left inset shows the period vs  $I_c R$ . Bottom right inset show the onset-to-period ratio  $\frac{H_{p0}}{\text{Period}}$  vs  $I_c R$ .

$V_{3f}$  is measured at the probe through a transmission line, which is lossy. Thus, a scaling factor for harmonic signal  $Y_{scale} = \frac{V_{3\omega}}{V_{3f}}$  is also required.

To uniquely relate experimental data at a temperature  $T$  to the RSJ calculation at a constant  $I_c R$ ,  $I_\omega R$  amplitudes corresponding to the dips in  $V_{3\omega}(I_\omega R)$  were identified and defined as  $H_{pn}(I_c R)$ . Then the procedure outlined in part A was used to calculate  $H_{p0}(I_c R)$  and the period from the data calculated from the RSJ model. Fig. S8 shows  $H_{p0}$  to  $H_{p10}$  vs  $I_c R$  calculated from the RSJ model. The period is found to be nearly constant as a function of  $I_c R$ .  $H_{p0}$  linearly decreases with  $I_c R$  and saturates at low  $I_c R$  values. This is consistent with the experimental data shown in Fig. S5, where  $H_{p0}$  saturates as  $T \rightarrow T_c$ . We find that the onset-to-period ratio  $\frac{H_{p0}}{\text{Period}}$  is a unique function of  $I_c R$  and does not depend on the choice of  $X_{scale}$ .

To calculate  $I_c R(T)$  of the junction, for every temperature the onset-to-period ratio  $\frac{H_{p0}}{\text{Period}}$  was calculated from the data. Then the unique value of  $I_c R$  corresponding to that onset-to-period ratio was identified. This procedure was then repeated for each measurement temperature to find  $I_c R(T)$ . Once  $I_c R(T)$  is known,  $X_{scale}(T)$  is calculated as the ratio of  $H_{p0}$  calculated from the RSJ model to  $H_{p0}$  calculated from the experimental data, while  $Y_{scale}(T)$  is left as a free fitting parameter.

As a next step, the Ambegaokar-Baratoff relations were used to estimate the superconducting gap  $\Delta(T)$

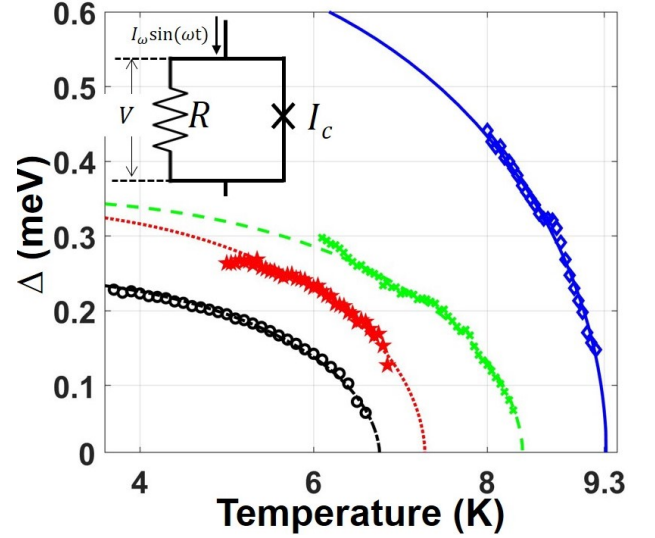

FIG. S9. Calculated superconducting gap at the weak-link vs temperature and BCS fit for Bulk Nb weak-link 1 (blue  $\diamond$  markers-solid line), Bulk Nb weak-link 2 (green  $\times$  markers-dashed line), Bulk Nb weak-link 3 (red  $\star$  markers-dotted line) and Nb on Cu (black circle markers-dash-dotted line).

from  $I_c R(T)$ :

$$I_c R(T) = \frac{\pi \Delta(T)}{2e} \tanh\left(\frac{\Delta(T)}{2k_B T}\right) \quad (\text{S4})$$

Finally, the temperature dependence of the superconducting gap  $\Delta(T)$  was fit to the temperature dependence of the gap predicted by BCS theory [5] and  $\Delta(0)$  was extracted (Fig. S9). The resulting fitting parameters are summarized in Table. S.I and Table. I of the main text.

| Sample                | Weak-Link Family | $\langle X_{scale} \rangle$<br>( $\mu\text{V}/\text{arb. units}$ ) | $\langle Y_{scale} \rangle$<br>( $n\text{V}/n\text{V}$ ) |
|-----------------------|------------------|--------------------------------------------------------------------|----------------------------------------------------------|
| Bulk Nb<br>from MSU   | 1                | 0.22                                                               | 68.56                                                    |
|                       | 2                | 0.12                                                               | 120                                                      |
|                       | 3                | 0.11                                                               | 125                                                      |
| Nb on Cu<br>from CERN | -                | 0.73                                                               | 22.85                                                    |

TABLE S.I. Summary of fit parameters for the 3 weak-links measured from large grain bulk Nb sample.

### C. TIME-DEPENDENT GINZBURG-LANDAU (TDGL) MODEL

The Ginzburg-Landau theory is a generic macroscopic quantum model appropriate for understanding the non-linear properties of superconductors. The Ginzburg-Landau model defines a complex-valued "order parameter"  $\Psi(\vec{r}, t)$  and the vector potential  $\vec{A}(\vec{r}, t)$ , where  $\vec{r}$  is

position and  $t$  is time. The order parameter is a measure

of the local strength of the superconducting state,

$$|\Psi(\vec{r}, t)|^2 = n_s(\vec{r}, t) \quad (S5)$$

Introducing some normalized quantities the time-dependent Ginzburg-Landau equations can be written in it's normalized form:

$$\eta \frac{\partial \tilde{\Psi}}{\partial t} = - \left( \frac{i}{\kappa} \vec{\nabla} + \kappa \vec{A} \right)^2 \tilde{\Psi} + (1 - |\tilde{\Psi}|^2) \tilde{\Psi} \quad (S6)$$

$$\tilde{\sigma} \frac{\partial \vec{A}}{\partial t} = \frac{1}{2\kappa^2 i} \left( \tilde{\Psi}^* \vec{\nabla} \tilde{\Psi} - \tilde{\Psi} \vec{\nabla} \tilde{\Psi}^* \right) - |\tilde{\Psi}|^2 \vec{A} - \vec{\nabla} \times \vec{\nabla} \times \vec{A} \quad (S7)$$

$$\vec{J} = \frac{1}{2\kappa^2 i} \left( \tilde{\Psi}^* \vec{\nabla} \tilde{\Psi} - \tilde{\Psi} \vec{\nabla} \tilde{\Psi}^* \right) - |\tilde{\Psi}|^2 \vec{A} \quad (S8)$$

Here  $\tilde{\Psi} = \frac{\Psi}{\Psi_\infty}$  where  $|\Psi_\infty|^2$  is the bulk superfluid density at zero temperature in the absence of external magnetic field.  $\tilde{x} = \frac{x}{\lambda_0}$  thus  $\vec{\nabla} = \lambda_0 \vec{\nabla}$  where  $x$  represents length and  $\lambda_0$  is the zero temperature GL penetration depth. Here  $\kappa = \frac{\lambda_0}{\xi_0}$  where  $\xi_0$  is the zero temperature GL coherence length.  $\tilde{T} = \frac{T}{T_c}$  where  $T_c$  is the critical temperature of the superconductor.  $\vec{\tilde{B}} = \frac{\vec{B}}{B_{c2}}$  where  $B_{c2} = \frac{\Phi_0}{\xi_0^2}$ .  $\vec{\tilde{A}} = \frac{\lambda_0}{\kappa^2 \Phi_0} \vec{A}$  where  $\Phi_0 = \frac{h}{2e}$  is the magnetic flux quantum.  $\vec{\tilde{J}} = \frac{\vec{J}}{J_c}$  where  $J_c = \frac{\mu_0 \lambda_0^3}{\kappa^2 \Phi_0} = \frac{B_{c2}}{\mu_0 \lambda_0}$  is the critical current density.  $\tilde{t} = \frac{t}{\tau_0}$  where  $\tau_0 = \mu_0 \lambda_0^2 \sigma_n$  is a characteristic time for the relaxation of  $\vec{A}$ .  $\eta = \frac{\tau_{GL}}{\tau_0}$  where  $\tau_{GL} = \frac{\xi_0^2}{D}$  and  $D$  here is the phenomenological electron diffusion coefficient given by  $D = \frac{v_F l}{3}$  [6] with  $v_F$  being the Fermi velocity and  $l$  being the quasi-particle mean free path [7].  $\tilde{\sigma} = \frac{\sigma}{\sigma_n}$ , where  $\sigma$  is the conductivity of non-superconducting current and  $\sigma_n$  is the normal state conductivity at 0K. From now on we will drop "  $\sim$  " from Eqs. S6-S8 for simplicity.

To numerically simulate the superconducting domain, we need to specify the boundary conditions. Any current passing through the boundary between a superconducting domain and vacuum/insulator would be nonphysical, thus on the boundary  $\partial\Omega$  of the superconducting domain  $\Omega$  we expect:

$$\vec{J} \cdot \hat{n} = 0 \quad \text{on} \quad \partial\Omega \quad (S9)$$

Here  $\hat{n}$  is unit vector normal to the boundary, and since we expect Eq.S8 to be true even when  $\vec{A} = 0$  and  $\Psi \neq 0$  the first boundary condition is:

$$\vec{\nabla} \Psi \cdot \hat{n} = 0 \quad \text{on} \quad \partial\Omega \quad (S10)$$

Likewise when both  $\vec{A} \neq 0$  and  $\Psi \neq 0$ , to satisfy S9:

$$|\Psi|^2 \vec{A} \cdot \hat{n} = 0 \quad \text{on} \quad \partial\Omega \quad (S11)$$

leading to

$$\vec{A} \cdot \hat{n} = 0 \quad \text{on} \quad \partial\Omega \quad (S12)$$

After reviewing some previously published TDGL simulations [8],[9], we noticed that generally Eq.S13 is enforced on the boundary as magnetic field continuity condition:

$$\vec{\nabla} \times \vec{A} = B_{\text{external}} \quad \text{on} \quad \partial\Omega \quad (S13)$$

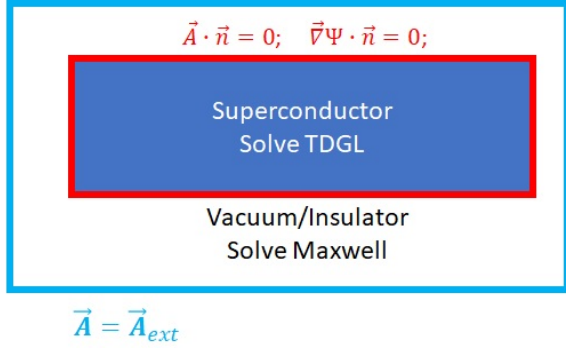

FIG. S10. Schematic illustration of the superconductor and vacuum domains and boundary conditions in TDGL simulation.

However this implies that the superconducting screening current has no effect on the magnetic field at the boundary and beyond the superconducting domain. This is physically incorrect in our case. The effect of screening currents is crucial when one is trying to simulate spatially nonuniform external magnetic field (like magnetic dipoles), and the resulting nonlinear response.

COMSOL multiphysics simulation software was used to numerically solve Eq.S6 and Eq.S7. Our simulation is divided into two domains: Superconductor and Vacuum (see Fig. 5(a)). The coupled TDGL equations are solved in the superconductor domain and only Maxwell's equations are solved in the vacuum domain with appropriate boundary conditions at the interface. Equations S10 and S12 were enforced at the superconductor/vacuum interface, while Eq.S13 was enforced at the outer boundary of the second domain where the contribution from the superconductor is negligible (assuming the second domain is large enough). Fig. S10 schematically represents this scenario.

The superconducting domain and vacuum domain are simulated inside two coaxial cylinders with equal radius  $R$  (see Fig. S11) and axis along the  $\hat{z}$  axis of the Cartesian coordinate system. The origin of this coordinate system is located on the superconductor surface immediately below the dipole. The height of the superconducting domain is  $h_{sc}$  and the height of the vacuum domain is  $h_{vac}$  in normalized units.

The RF magnetic field produced by the magnetic writer probe sitting on top of a sample is very similar to the magnetic field produced by a horizontal point magnetic dipole with normalized magnetic moment  $M_{dp}(t) \parallel \hat{x}$  placed at a height  $h_{dp}$  above the sample. The normalized vector potential produced by such a dipole in free space

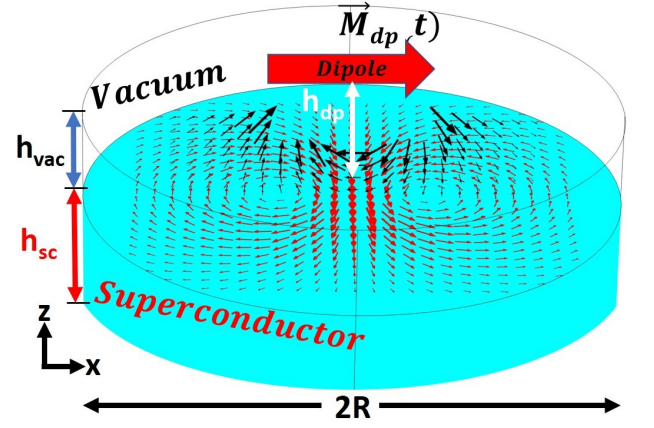

FIG. S11. TDGL simulation setup. The magnetic probe is approximated as an oscillating point magnetic dipole parallel to the surface. Red Arrows: Surface currents on the horizontal superconductor/vacuum interface. Black Arrows: Magnetic field on a vertical plane perpendicular to the superconductor surface and including the dipole.

is given by:

$$\vec{A}_{dp}(x, y, z, t) = \frac{M_{dp}(t)}{(x^2 + y^2 + (z - h_{dp})^2)^{3/2}} \left( -(z - h_{dp})\hat{y} + y\hat{z} \right) \quad (\text{S14})$$

Thus, for the purposes of this simulation, the magnetic writer probe can be mathematically approximated to be a horizontal point magnetic dipole. In the simulation, we specify  $M_{dp}(t)$  indirectly through the magnetic field at the origin  $\vec{B}_0(t) = \vec{\nabla} \times \vec{A}_{dp}(0, 0, 0, t) = -\frac{M_{dp}(t)}{h_{dp}^3} \hat{x}$ .

Fig. S12 shows a simulation which was done with  $R = 12$ ,  $h_{sc} = 6$ ,  $h_{vac} = 3$ ,  $\eta = 1.675$ ,  $h_{dp} = 8$ ,  $\vec{B}_0 = 0.75 \sin(\omega t)$ ,  $T = 0$  and  $\frac{2\pi}{\omega} = 200\tau_0$ . The simulation was run for 3 driving periods to stabilize and the results shown in Fig. S12 are from the 4<sup>th</sup> period. We see that as  $\vec{B}_0(t)$  increases a suppressed  $|\Psi|^2$  domain forms at the superconductor surface immediately below the dipole. At  $t = 50\tau_0$  the magnetic field reaches its peak value and the suppressed superconducting region reaches its deepest point inside the superconducting domain. Later ( $t > 50\tau_0$ ), the amplitude of magnetic field decreases, the normal state domain vanishes and vortex semi-loops emerge from it, move back towards the surface and vanish there before the end of the first half of the RF cycle. In the second part of the RF cycle, the same process is repeated but now antivortex-semiloops enter the superconducting domain. In this scenario vortices and anti-vortices never meet, unlike the situation discussed in [10].

The response RF magnetic field at the location of the dipole  $\vec{B}_{sc}(t)$  was calculated from the time-dependent

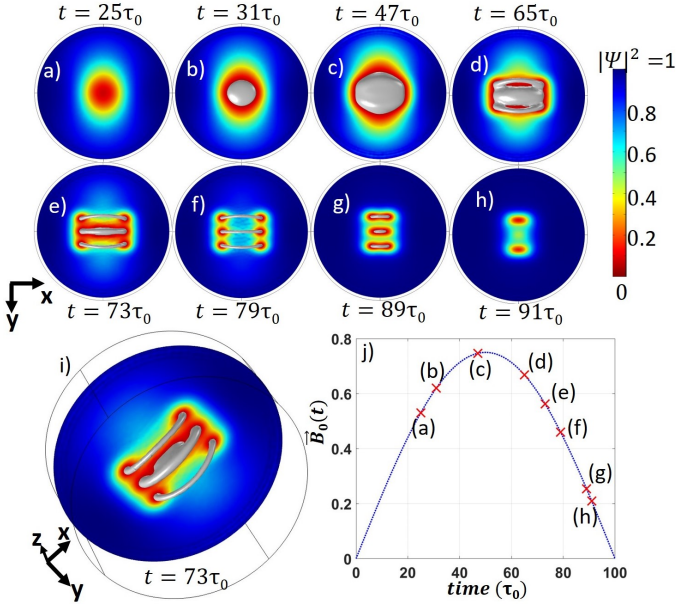

FIG. S12. a-h) Plots of  $|\Psi|^2$  evaluated at the superconductor surface at different times for an oscillating parallel magnetic dipole above the superconductor. In this view, one is looking from inside the superconducting domain into the vacuum domain.  $\vec{M}_{dp}(t)$  is chosen such that  $\vec{B}_0(t) = 0.75\sin(\omega t)\hat{x}$ . i) Same result as shown in Fig. S12.e) but in three dimensions from a different angle. Silver surfaces (corresponding to  $|\Psi|^2 = 0.005$ ) show the vortex semiloops. j)  $\vec{B}_0(t)$  at the surface vs time during the first half of the RF cycle. Red crosses correspond to field values for snapshots a-h.

screening currents. This calculation is simplified due to the symmetric nature of the problem. At the location of the dipole, magnetic field produced by the superconductor is only in the  $\hat{x}$  direction. The third harmonic response  $V_{3f}(B_0)$  was obtained through Fourier transformation of  $\vec{B}_{sc}(t)$ .  $V_{3f}(B_0)$  as a function of the peak magnetic moment of the dipole shows the following behaviour. Harmonic response is small for small moments but increases rapidly above an onset magnetic moment, reaches a peak value and then slowly decreases back to a finite value, which depends on temperature, height of the dipole and  $\eta$ . Note that this evolution is very similar to the low  $H_{rf} < H_{p0}$  part of the data shown in Fig.4 of the main text.

Many simulations were performed by varying the parameters listed in Table S.II. The radius of the simulation domain  $R$ , the height of the superconductor domain  $h_{sc}$  and the height of the vacuum domain  $h_{vac}$  control the geometry and some finite size effects can be seen for  $R < 30\lambda_0$  (Fig. S13). However, at sufficiently high values of  $R$ ,  $h_{sc}$  and  $h_{vac}$ , the third harmonic response  $V_{3f}$  is independent of the simulation size. Note that larger

| Parameter Name                          | Symbol        | Range             |
|-----------------------------------------|---------------|-------------------|
| Temperature                             | $T$           | $0 - 0.95T_c$     |
| Applied RF field amplitude              | $B_0$         | $0.01-2 B_{c2}$   |
| Period of Applied RF field              | $2\pi/\omega$ | $100-2000 \tau_0$ |
| Dipole height                           | $h_{dp}$      | $2-12 \lambda_0$  |
| Radius of the simulation domain         | $R$           | $5-50 \lambda_0$  |
| Height of superconducting domain        | $h_{sc}$      | $3-20 \lambda_0$  |
| Height of vacuum domain                 | $h_{vac}$     | $6-30 \lambda_0$  |
| Ginzburg-Landau parameter               | $\kappa$      | $0.8-1$           |
| The ratio of characteristic time scales | $\eta$        | $0.1-10$          |

TABLE S.II. The parameters and range of values used for TDGL simulations of the oscillating magnetic dipole above the superconductor.

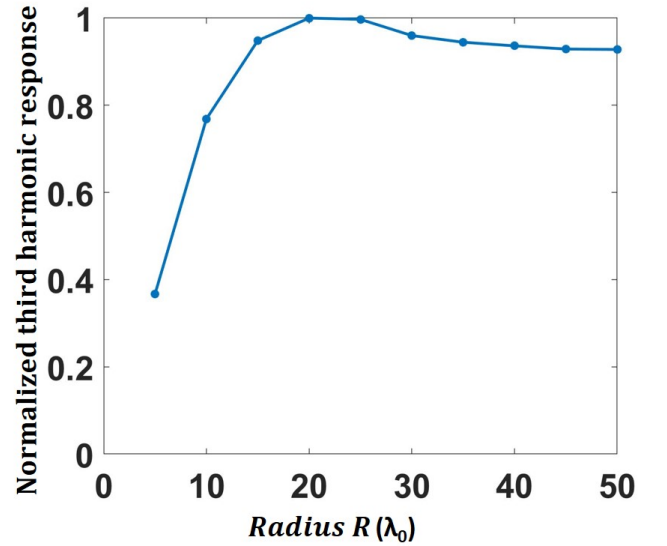

FIG. S13. The third harmonic response  $B_{3f}(B_0)$  normalized by the maximum value vs the radius of the simulation domain  $R$ . Note that  $h_{sc}$  and  $h_{vac}$  are varied proportionally with  $R$ .

geometry size leads to larger meshes and longer run times due to limited computational power.

In conclusion, the TDGL model can be used to describe the "pedestal" low-field non-periodic part of the third harmonic data measured from Nb samples, however no periodic response was observed from this model within the range of parameters that were used in our simulations.

\* Corresponding author: bakhromtjk@gmail.com

- [1] P. Dhakal, S. Chetri, S. Balachandran, P. J. Lee, and G. Ciovati, Phys. Rev. Accel. Beams **21**, 032001 (2018).
- [2] S. Wilde, R. Valizadeh, O. B. Malyshev, G. B. G. Sten-

- ning, T. Sian, and B. Chesca, Phys. Rev. Accel. Beams **21**, 073101 (2018).
- [3] A.-M. Valente-Feliciano, *Development of SRF thin film materials for monolayer/multilayer approach to increase the performance of SRF accelerating structures beyond bulk Nb*, Ph.D. thesis, Universit Paris (2014).
- [4] J. McDonald and J. R. Clem, Phys. Rev. B **56**, 14723 (1997).
- [5] M. Tinkham, *Introduction to superconductivity*, 2nd ed. (Dover Publications, Inc., Mineola, New York, 2004) Chap. 3, p. 63.
- [6] M. Cyrot, Reports on Progress in Physics **36**, 103 (1973).
- [7] I. S. Aranson, N. B. Kopnin, and V. M. Vinokur, Phys. Rev. B **63**, 184501 (2001).
- [8] T. S. Alstrøm, M. P. Sørensen, N. F. Pedersen, and S. Madsen, Acta Applicandae Mathematicae **115**, 63 (2011).
- [9] W. D. Gropp, H. G. Kaper, G. K. Leaf, D. M. Levine, M. Palumbo, and V. M. Vinokur, Journal of Computational Physics **123**, 254 (1996).
- [10] T. Tai, *Measuring Electromagnetic Properties of Superconductors in High and Localized RF Magnetic Field*, Ph.D. thesis, University of Maryland (2013), available at <https://drum.lib.umd.edu/handle/1903/14668>.
